# Supplementary material for: HyperSegNAS: Bridging One-Shot Neural Architecture Search with 3D Medical Image Segmentation using HyperNet
Source: arXiv:2112.10652 source file (2022-03-24)
Supplement: Supplementary file 2 [file supplemental_vis.tex]

\begin{figure*}[!htb]
    \setlength{\tabcolsep}{0.2pt}
    \begin{tabular}[b]{cc}
        \begin{subfigure}[t]{0.5\linewidth}
            \includegraphics[width=\textwidth]{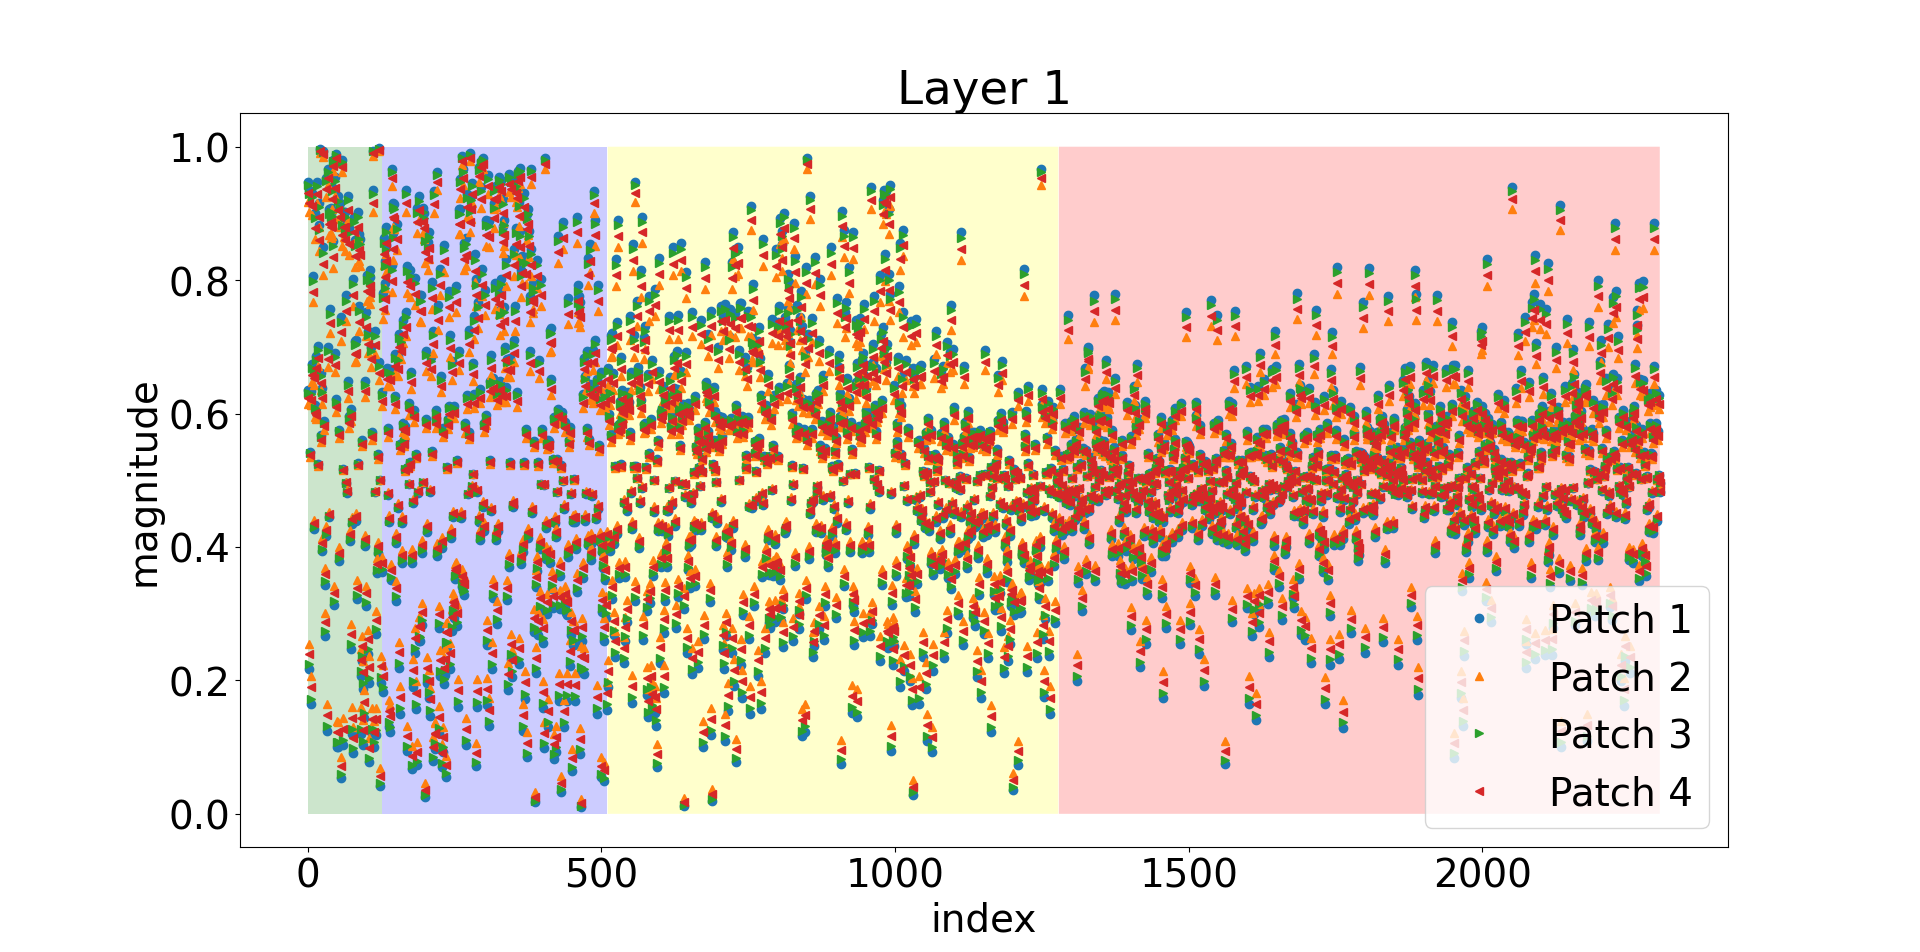}
            \caption{$\omega^{a,I}_{\mathcal{H}_\theta}$ at layer $l=1$ on \underline{background} patches.}
        \end{subfigure} &
        \begin{subfigure}[t]{0.5\linewidth}
            \includegraphics[width=\textwidth]{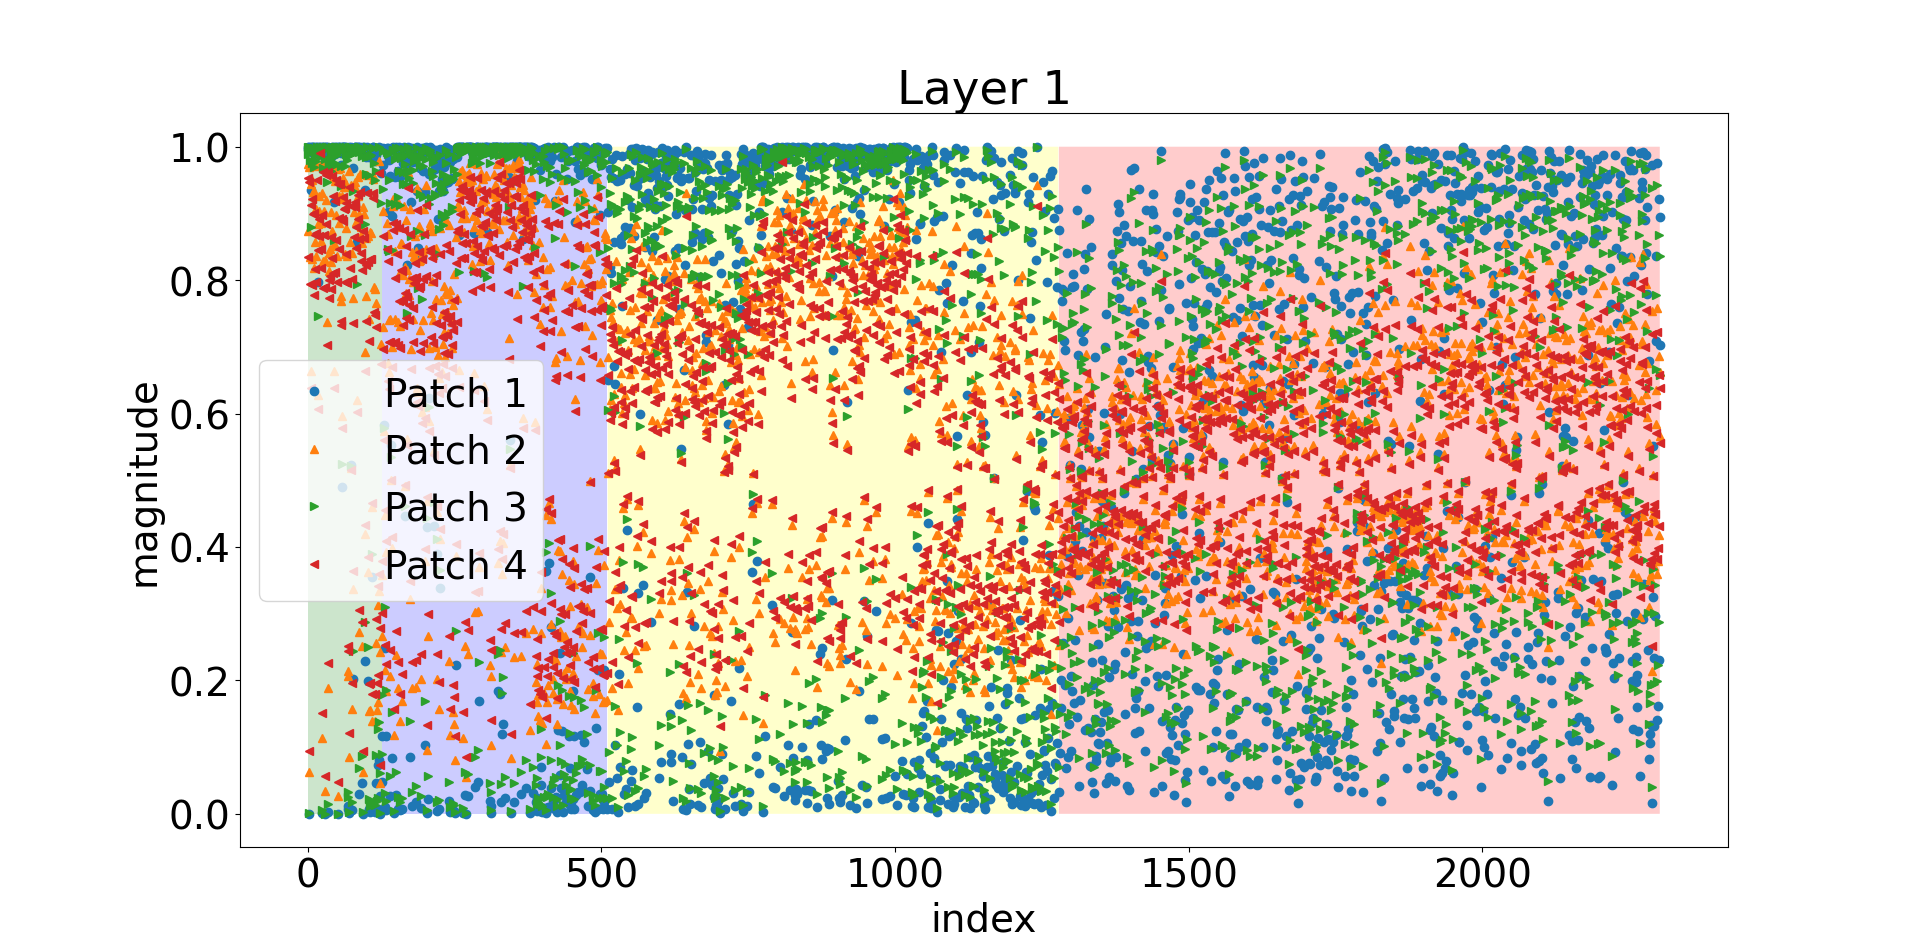}
            \caption{$\omega^{a,I}_{\mathcal{H}_\theta}$ at layer $l=1$ on \underline{foreground} patches.}
        \end{subfigure} 
        \\
        \begin{subfigure}[t]{0.5\linewidth}
            \includegraphics[width=\textwidth]{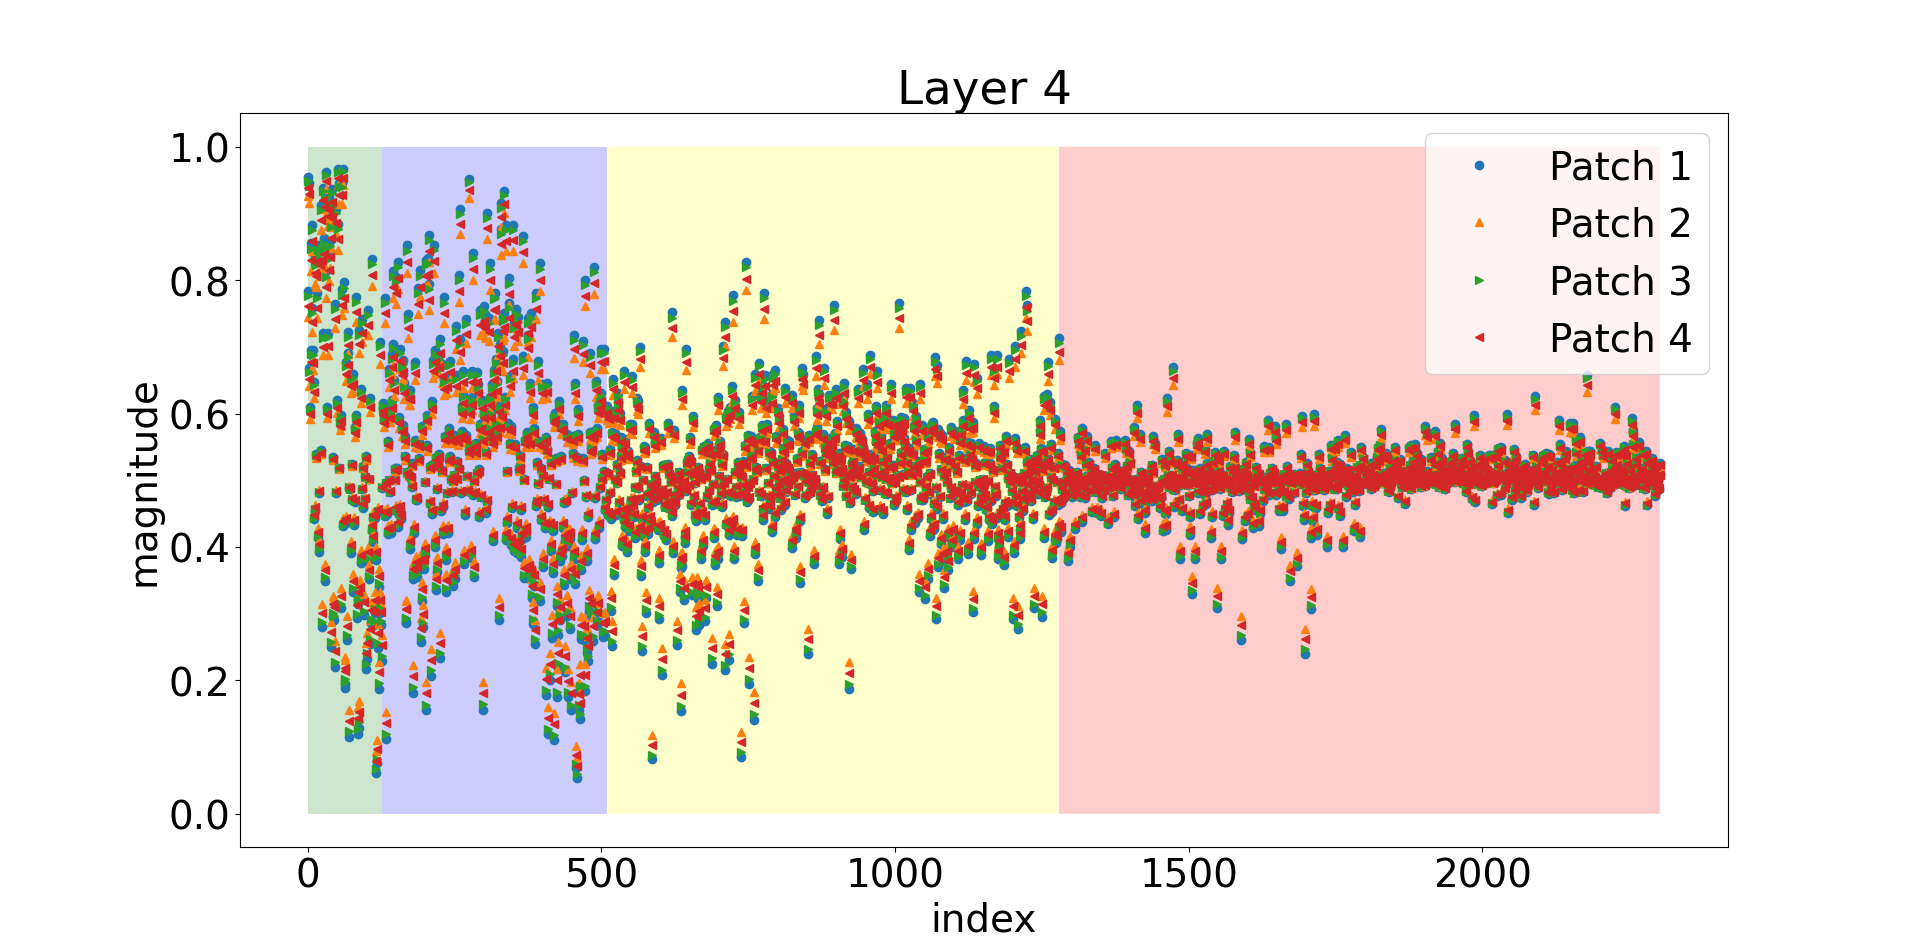}
            \caption{$\omega^{a,I}_{\mathcal{H}_\theta}$ at layer $l=4$ on \underline{background} patches.}
        \end{subfigure} &
        \begin{subfigure}[t]{0.5\linewidth}
            \includegraphics[width=\textwidth]{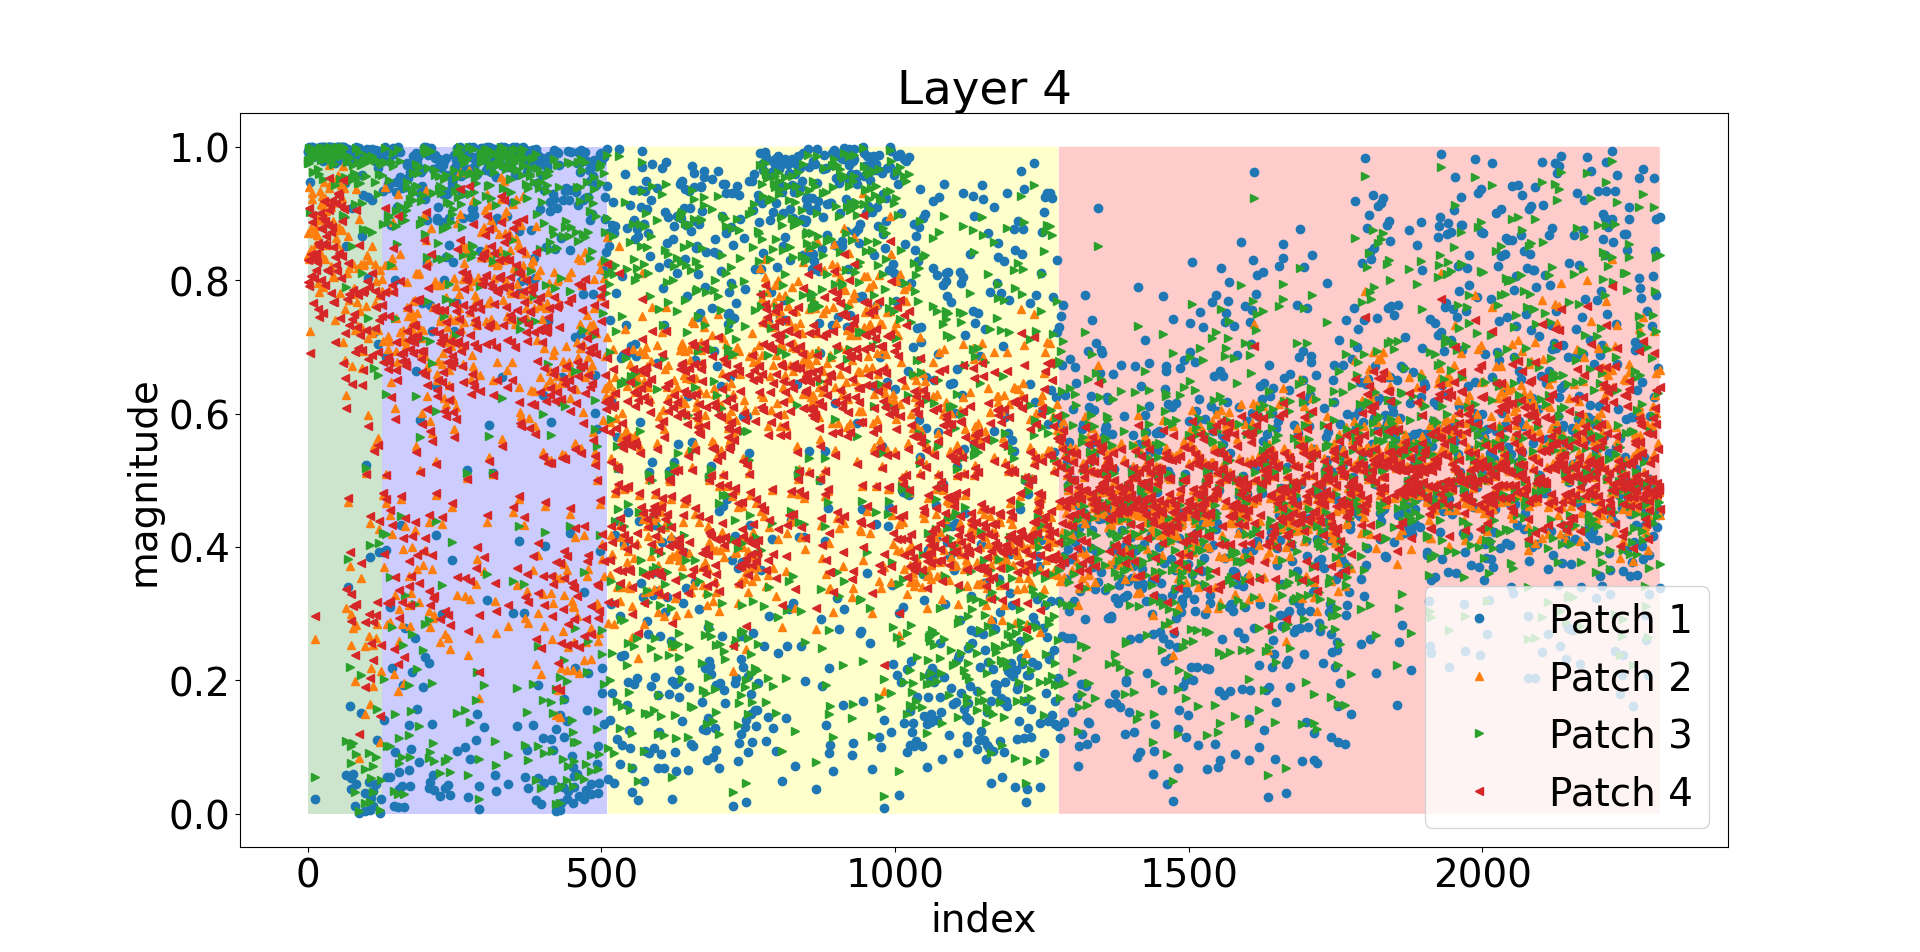}
            \caption{$\omega^{a,I}_{\mathcal{H}_\theta}$ at layer $l=4$ on \underline{foreground} patches.}
        \end{subfigure}  
        \\
        \begin{subfigure}[t]{0.5\linewidth}
            \includegraphics[width=\textwidth]{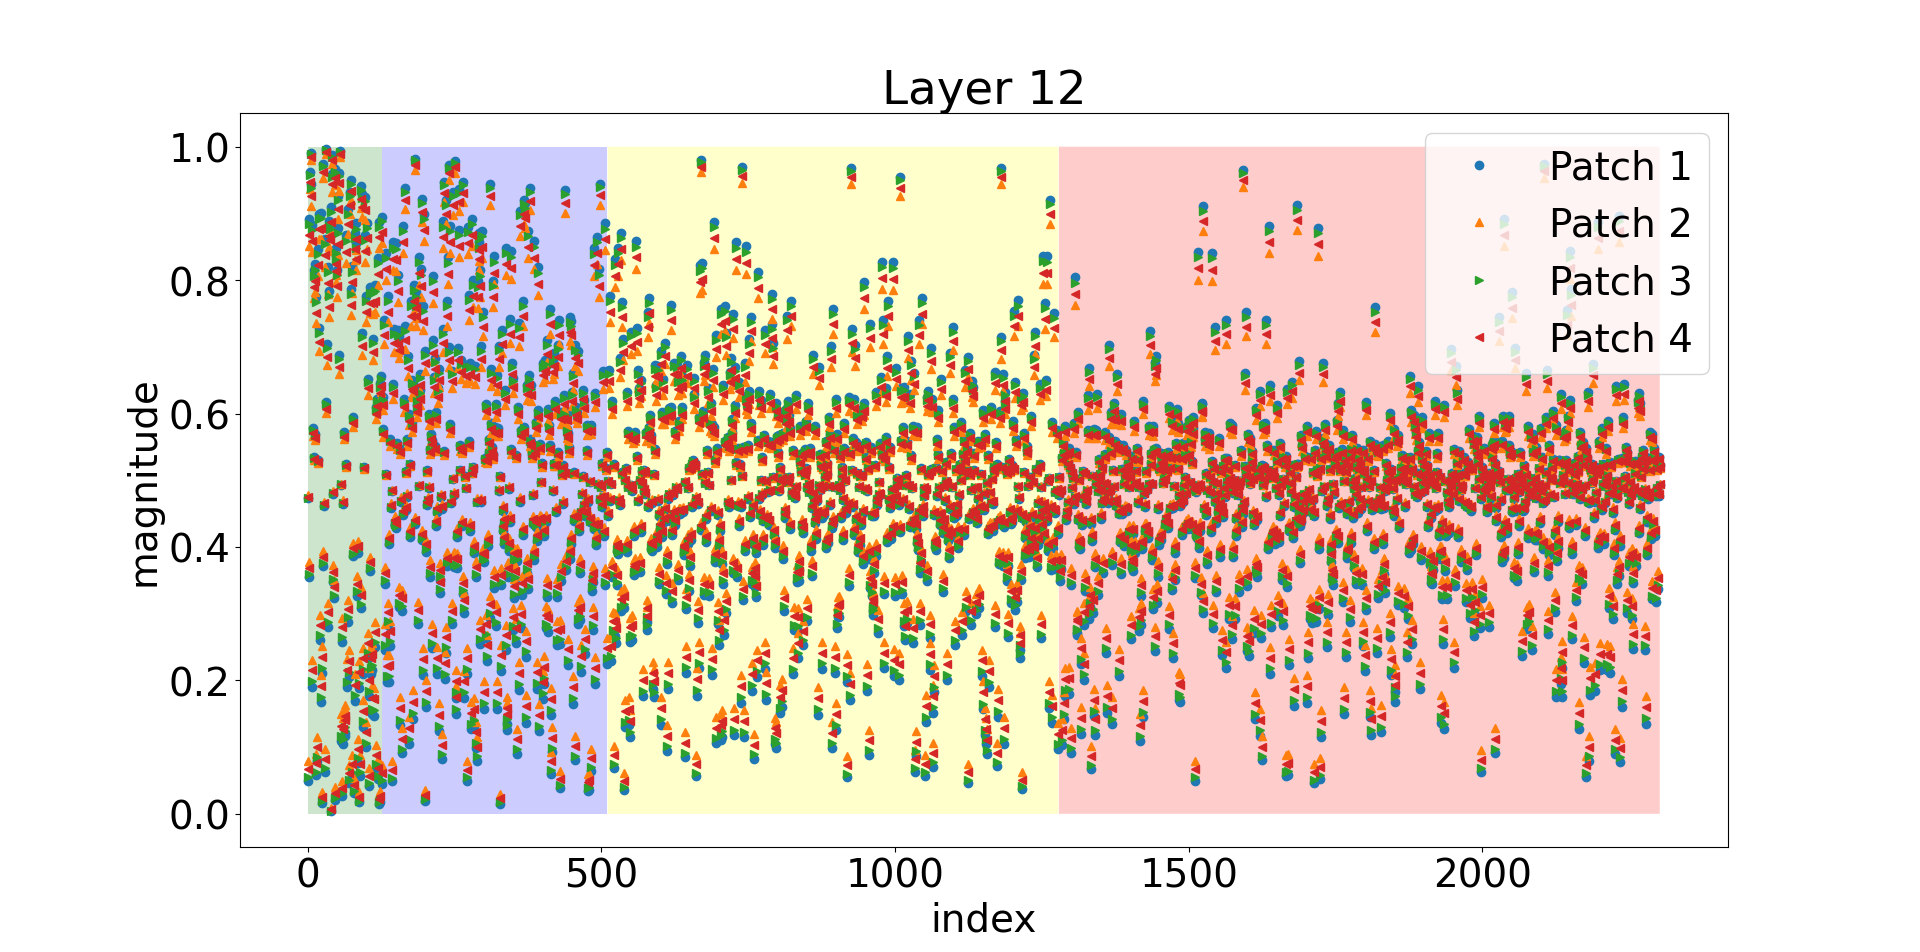}
            \caption{$\omega^{a,I}_{\mathcal{H}_\theta}$ at layer $l=12$ on \underline{background} patches.}
        \end{subfigure} &
        \begin{subfigure}[t]{0.5\linewidth}
            \includegraphics[width=\textwidth]{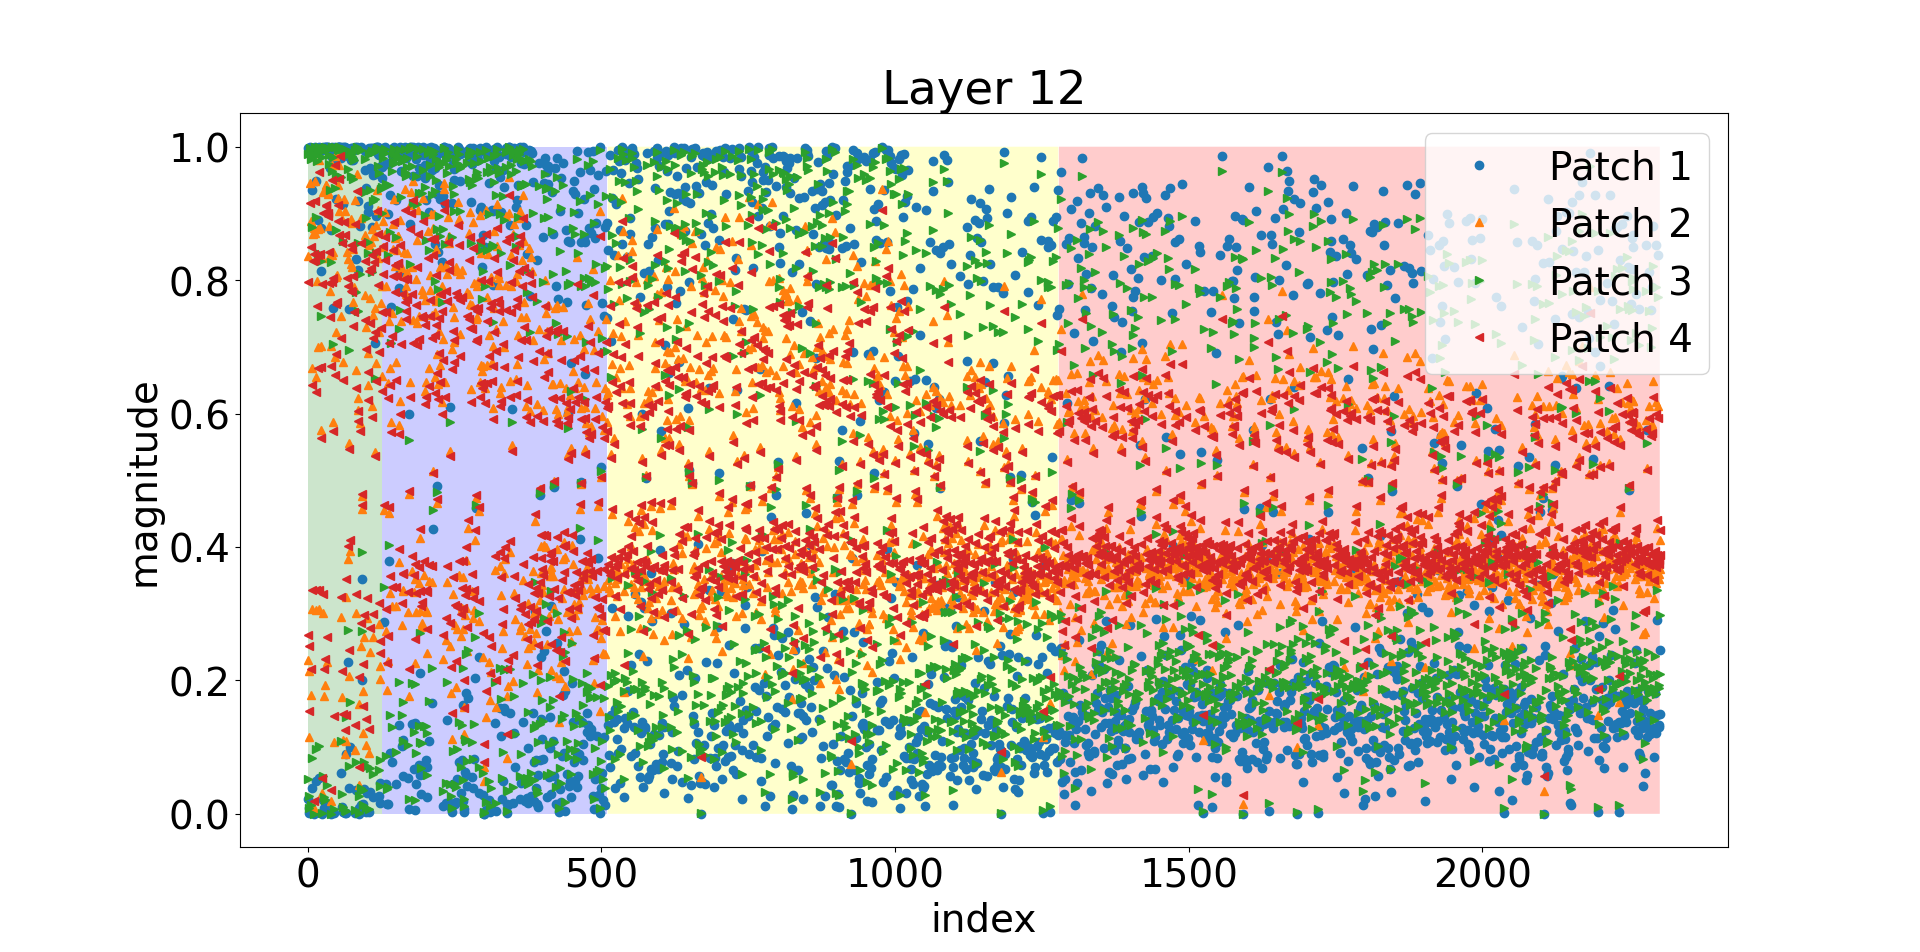}
            \caption{$\omega^{a,I}_{\mathcal{H}_\theta}$ at layer $l=12$ on \underline{foreground} patches.}
        \end{subfigure} \\
    \end{tabular}
    \caption{Visualization of $\omega^{a_i,I_i}_{\mathcal{H}_\theta}$ generated from $\mathcal{H}$. The weights within the green regions correspond to the highest resolution features, $F^{l}_{\downarrow 2}$, the blue region corresponds to weights for $F^{l}_{\downarrow 4}$, the yellow region corresponds to weights for $F^{l}_{\downarrow 8}$, and the red region corresponds to weights for $F^{l}_{\downarrow 16}$. Clear differences can be observed between weights generated from foreground and background patches.}
    \label{fig:atten_vis}
    \vspace{-1em}
\end{figure*}
