# Supplementary material for: HyperSegNAS: Bridging One-Shot Neural Architecture Search with 3D Medical Image Segmentation using HyperNet
Source: arXiv:2112.10652 source file (2022-03-24)
Supplement: Supplementary file 3 [file supplemental.tex]

\appendix

\section{Algorithm Overview}

\begin{algorithm}[!htb]
\SetAlgoLined
\textbf{Networks:} image encoder: $\mathcal{M}$, Meta-Assistant Network: $\mathcal{H}$, super-net: $\mathcal{F}$\\
\KwIn{sampled input image: $I_i\in\mathbb{R}^{96\times96\times96}$, sampled architecture: $a_i\in\mathbb{N}^{L\times E\times O}$, ground truth: $S_{gt}\in\mathbb{N}^{96\times96\times96}$, total layers: $L=12$, total edges between columns: $E=10$, total operations: $O=2$, super-net training iter.: $N_1=160000$, annealing training iter.: $N_2=20000$}
\KwOut{segmentation mask: $S\in\mathbb{N}^{96\times96\times96}$}
\For{$i=1$ \KwTo $N_1$}{
 $l_{\textrm{image}}=\mathcal{M}(I_i)$\\
 $l_{\textrm{arch}}=\mathrm{flatten}(a_i)$\\
 $\omega^{a_i,I_i}_{\mathcal{H}_\theta}$ = $\mathcal{H}(l_{\textrm{arch}}\oplus l_{\textrm{image}})$\\
 $\omega_\textrm{active} = \omega^{a_i,I_i}_{\mathcal{H}_\theta}(l,e,c)*\omega_a(l,e,c)$\\
 $S = \mathcal{F}(I_i;a_i, \omega_\textrm{active})$\\
 $\mathcal{L}_{\textrm{train}}(S,S_{gt}) = \mathcal{L}_{\textrm{dice}}(S,S_{gt}) + \mathcal{L}_{\textrm{ce}}(S,S_{gt})$\\
 $\omega_\textrm{active}:=\omega_\textrm{active}-\alpha\frac{\delta \mathcal{L}_{\textrm{train}}}{\delta \omega_\textrm{active}}$
}

\For{$i=1$ \KwTo $N_2$}{
 $l_{\textrm{image}}=\mathcal{M}(I_i)$\\
 $l_{\textrm{arch}}=\mathrm{flatten}(a_i)$\\
 $\omega^{a_i,I_i}_{\mathcal{H}_\theta}$ = $\mathcal{H}(l_{\textrm{arch}}\oplus l_{\textrm{image}})$\\
 $\lambda = \frac{i}{N_2}$\\
 $\omega_\textrm{active} = (\lambda\omega_{\textrm{fixed}}+(1-\lambda)\omega^{a_i,I_i}_{\mathcal{H}_\theta})*\omega_a)$\\
 $S = \mathcal{F}(I_i;a_i, \omega_\textrm{active})$\\
 $\mathcal{L}_{\textrm{train}}(S,S_{gt}) = \mathcal{L}_{\textrm{dice}}(S,S_{gt}) + \mathcal{L}_{\textrm{ce}}(S,S_{gt})$\\
 $\omega_\textrm{active}:=\omega_\textrm{active}-\alpha\frac{\delta \mathcal{L}_{\textrm{train}}}{\delta \omega_\textrm{active}}$
}
 \caption{HyperSegNAS Training}
 \label{alg:Training}
\end{algorithm}

We provide a detailed description of the training pipeline for HyperSegNAS in Algorithm~\ref{alg:Training}, which includes training the super-net with $\mathcal{H}$ in $N_1$ iterations and annealing away $\mathcal{H}$ in $N_2$ iterations. For clarity, we denote the super-net as $\mathcal{F}(*;a,\omega_a)$, where the forward function involves the inferenced architecture and the corresponding weights. The $\textrm{flatten}(*)$ function converts the one-hot architecture matrix $a\in\mathbb{N}^{L\times E\times O}$ to the vector $l_{\textrm{arch}}\in\mathbb{N}^{L \cdot E}$, where each element in $l_{\textrm{arch}}$ indicates either inactive, a skip connection, or a $3\times 3\times 3$ convolution. Training loss is based on an equal combination of dice and cross-entropy loss. The super-net training schedule is similar to DiNTS~\cite{DBLP:conf/cvpr/He0RZX21}, where we use 1000 iterations for warm-up, during which the learning rate $\alpha$ linearly increases from 0.025 to 0.2. After warm-up, learning rate decreases by half at 20\%, 40\%, 60\%, and 80\% of $N_1$. During annealing, the learning rate is fixed at 0.0016. Similarly, during quick fine-tuning over individual architectures, learning rate is fixed at 0.0016. The architectures are fine-tuned over 5000 iterations.

\section{Network Architecture}

We provide the network architectures of the image encoder $\mathcal{M}$ and the Meta Assistant Network (MAN) in Table~\ref{table:M} and Table~\ref{table:H}. In the network tables, $N_c$ denotes the number of output channels, $C'$ denotes the channel dimension of generated features $F^{LR}$. We use `K\#-C\#-S\#-P\#' to denote the configuration of the convolution layers, where `K', `C', `S' and `P' stand for the kernel, input channel, stride and padding size, respectively.

\begin{table}[htb!]
\centering 
\begin{tabular}{l | c | l}
Name & $N_{c}$ & Description \\
\hline
INPUT & $1$ & Input $I$\\ 
CONV0 & $16$ & K3-C1-S2-P1 \\
IN & & InstanceNorm3d \\
RELU &  & \\
CONV1 & $32$ & K3-C16-S2-P1 \\
IN & & InstanceNorm3d \\
RELU &  & \\
CONV2 & $64$ & K3-C32-S2-P1 \\
IN & & InstanceNorm3d \\
RELU &  & \\
CONV3 & $128$ & K3-C64-S2-P1 \\
IN & & InstanceNorm3d \\
RELU &  & \\
CONV4 & $256$ & K3-C128-S2-P1 \\
IN & & InstanceNorm3d \\
RELU &  & \\
CONV5 & $256$ & K3-C256-S1-P0 \\
RELU &  & \\
\midrule
\end{tabular}
\caption{Network architecture of $\mathcal{M}$.}
\label{table:M}
\end{table}

\begin{table}[htb!]
\centering 
\begin{tabular}{l | c | l}
Name & $N_{c}$ & Description \\
\hline
INPUT & $378$ & Input $l_{\textrm{arch}}\oplus l_{\textrm{image}}$\\ 
FC0 & $2048$ & C378 \\
RELU &  & \\
FC1 & $4096$ & C2048 \\
RELU &  & \\
FC2 & $8192$ & C4096 \\
RELU &  & \\
FC3 & $16384$ & C8192 \\
RELU &  & \\
FC4 & $27648$ & C16384 \\
SIGMOID &  & \\
\midrule
\end{tabular}
\caption{Network architecture of $\mathcal{H}$.}
\label{table:H}
\end{table}

\begin{figure*}[!htb]
    \setlength{\tabcolsep}{0.2pt}
    \begin{tabular}[b]{cc}
        \begin{subfigure}[t]{0.5\linewidth}
            \includegraphics[width=\textwidth]{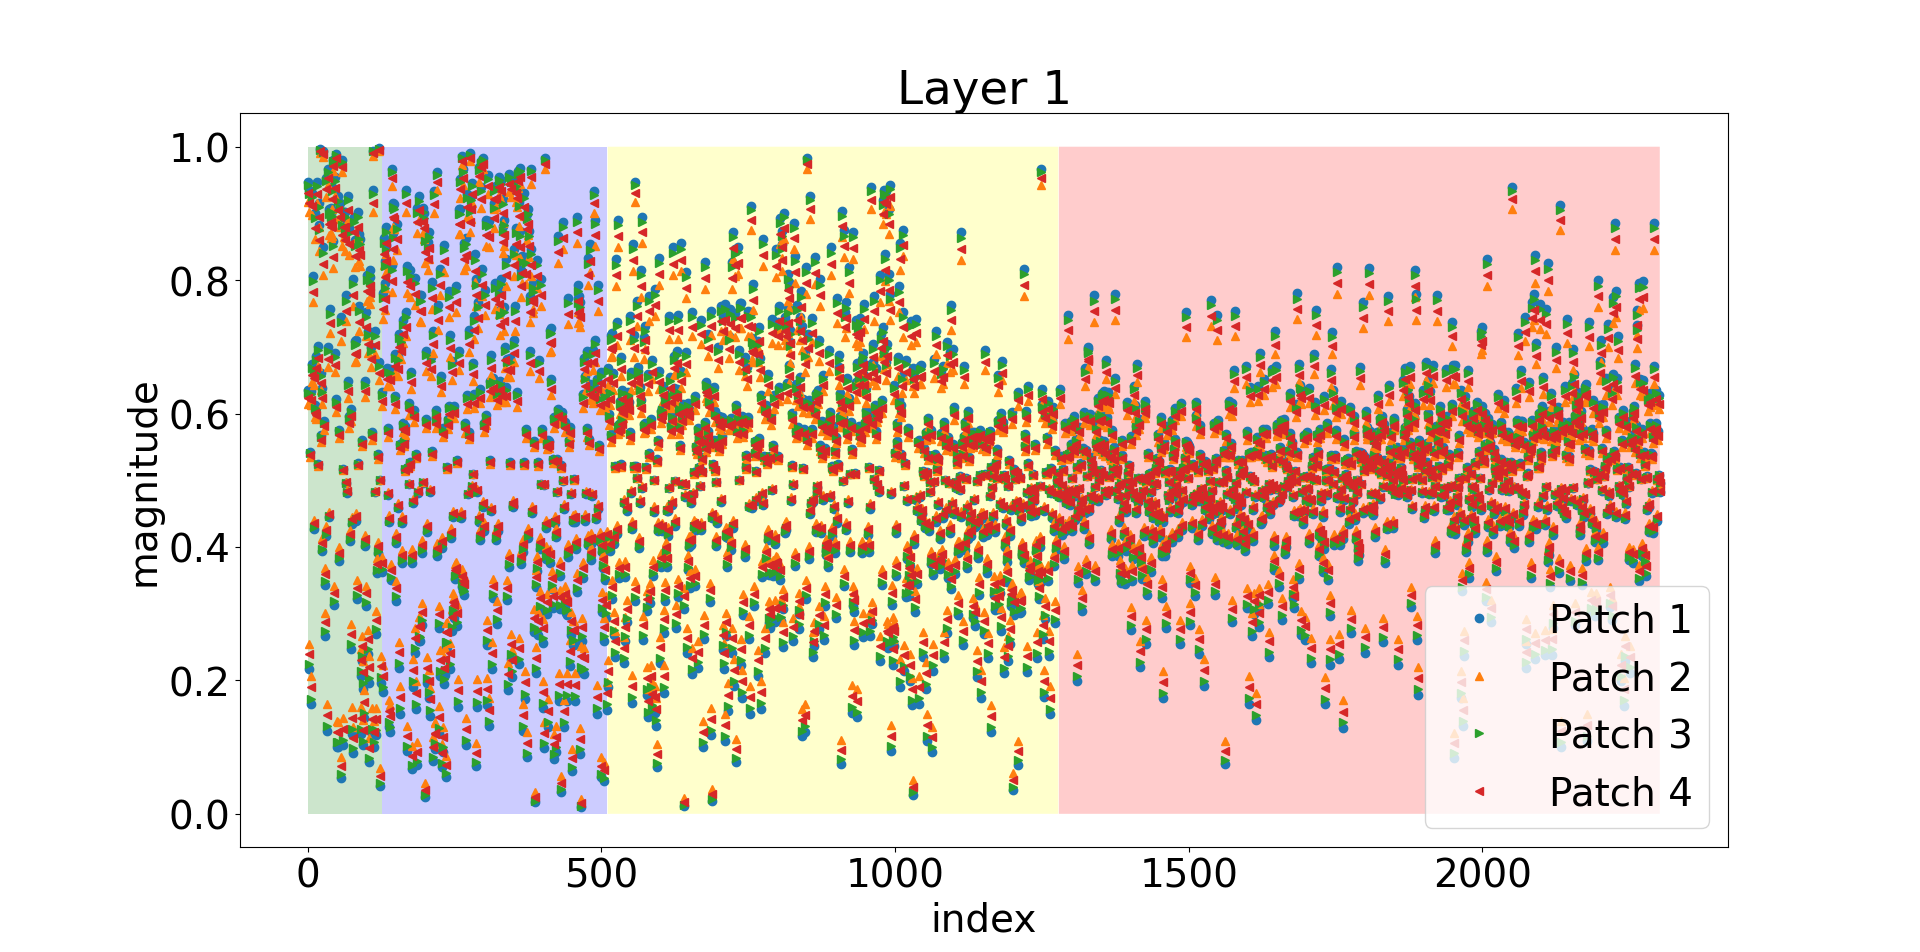}
            \caption{$\omega^{a,I}_{\mathcal{H}_\theta}$ at layer $l=1$ on \underline{background} patches.}
        \end{subfigure} &
        \begin{subfigure}[t]{0.5\linewidth}
            \includegraphics[width=\textwidth]{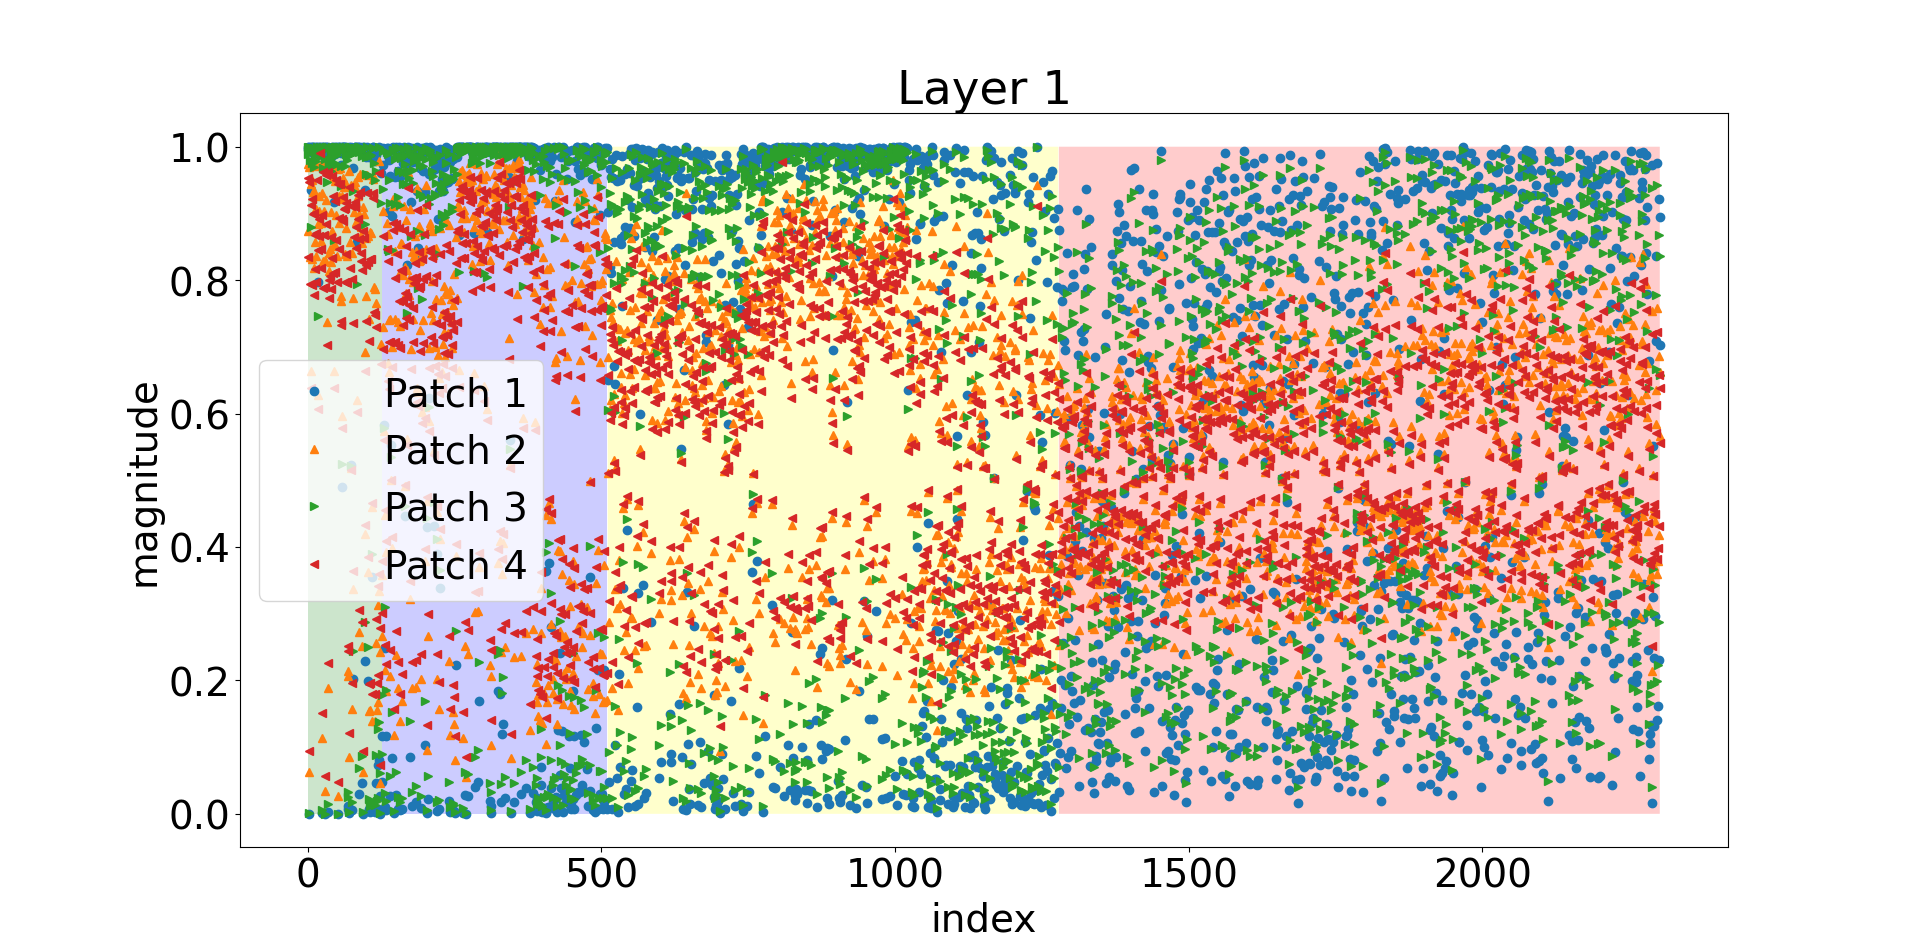}
            \caption{$\omega^{a,I}_{\mathcal{H}_\theta}$ at layer $l=1$ on \underline{foreground} patches.}
        \end{subfigure} 
        \\
        \begin{subfigure}[t]{0.5\linewidth}
            \includegraphics[width=\textwidth]{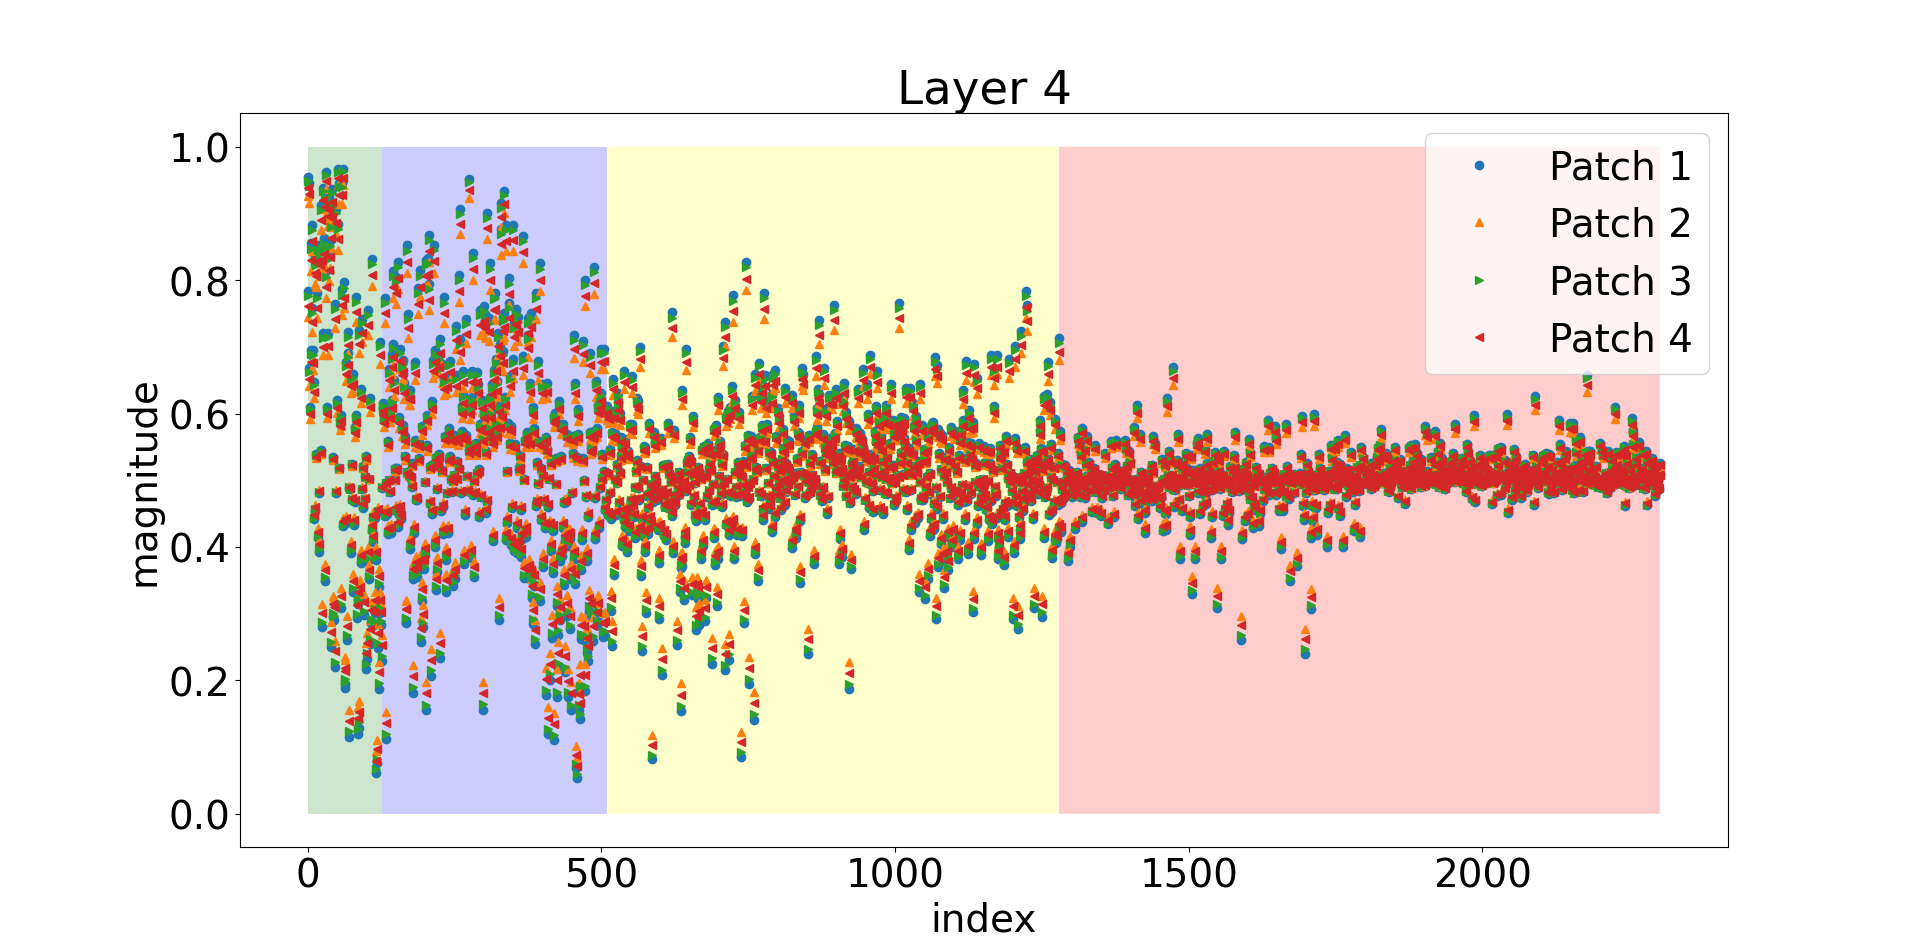}
            \caption{$\omega^{a,I}_{\mathcal{H}_\theta}$ at layer $l=4$ on \underline{background} patches.}
        \end{subfigure} &
        \begin{subfigure}[t]{0.5\linewidth}
            \includegraphics[width=\textwidth]{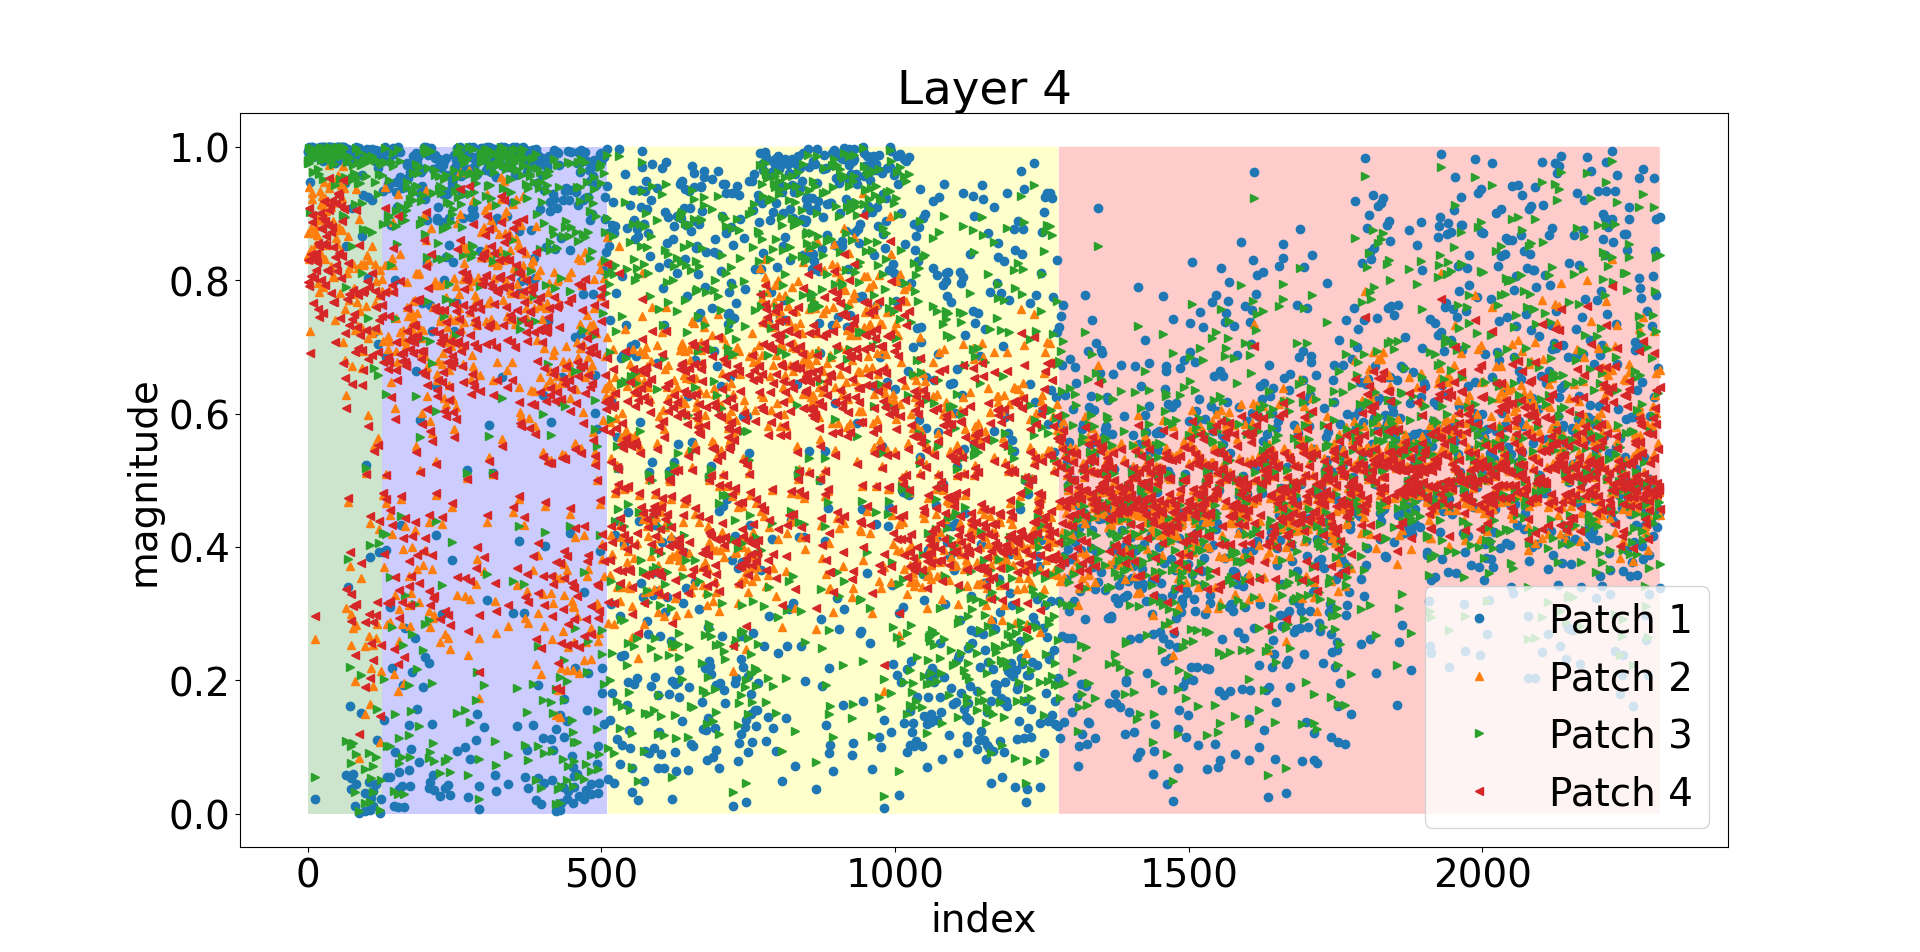}
            \caption{$\omega^{a,I}_{\mathcal{H}_\theta}$ at layer $l=4$ on \underline{foreground} patches.}
        \end{subfigure}  
        \\
        \begin{subfigure}[t]{0.5\linewidth}
            \includegraphics[width=\textwidth]{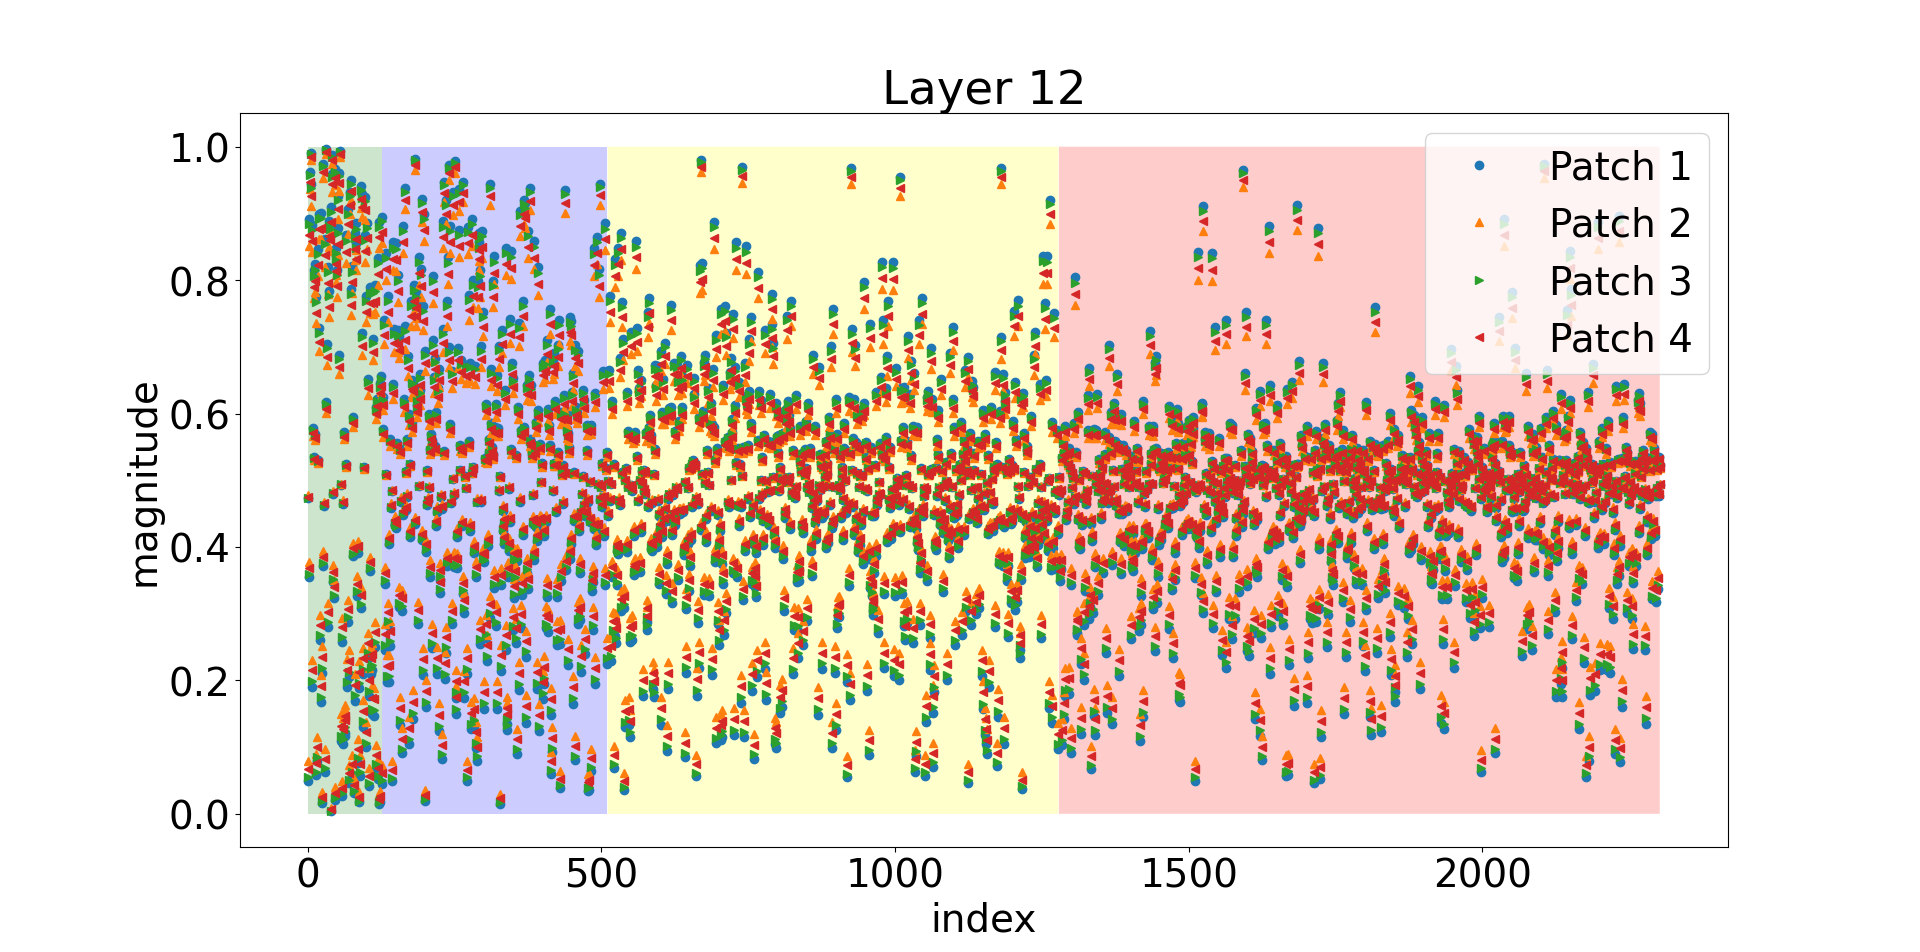}
            \caption{$\omega^{a,I}_{\mathcal{H}_\theta}$ at layer $l=12$ on \underline{background} patches.}
        \end{subfigure} &
        \begin{subfigure}[t]{0.5\linewidth}
            \includegraphics[width=\textwidth]{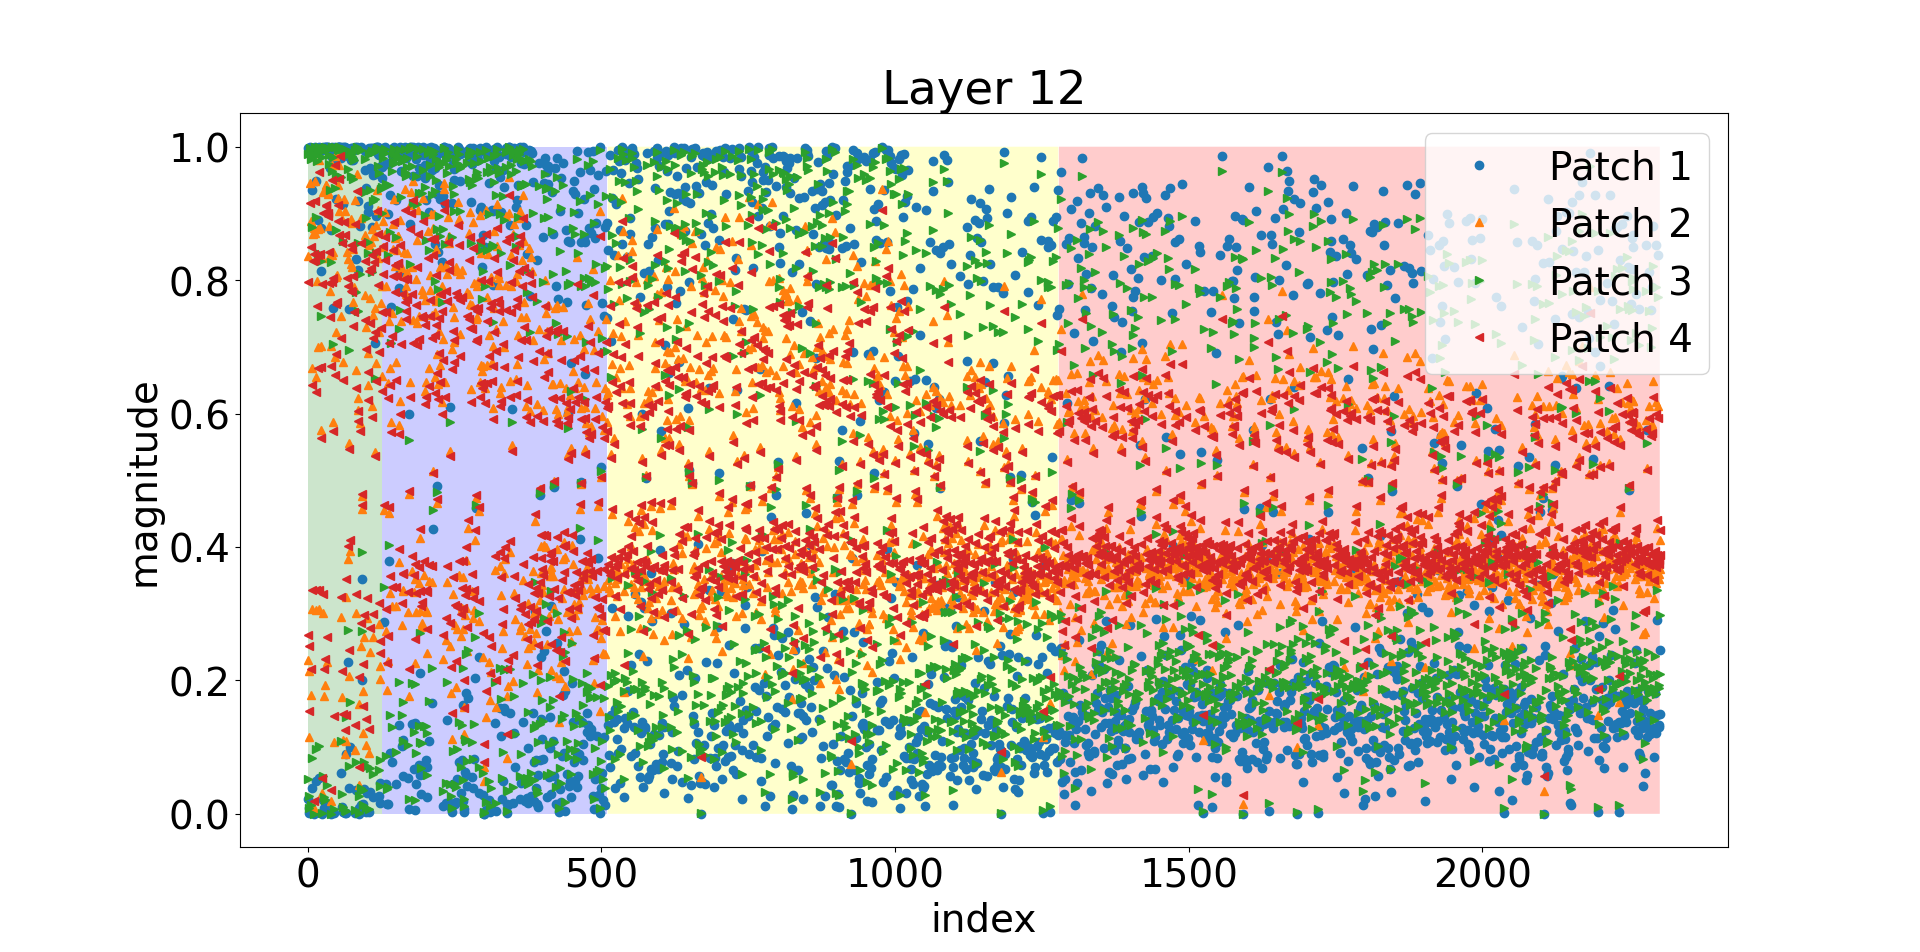}
            \caption{$\omega^{a,I}_{\mathcal{H}_\theta}$ at layer $l=12$ on \underline{foreground} patches.}
        \end{subfigure} \\
    \end{tabular}
    \caption{Visualization of $\omega^{a_i,I_i}_{\mathcal{H}_\theta}$ generated from $\mathcal{H}$. The weights within the green regions correspond to the highest resolution features, $F^{l}_{\downarrow 2}$, the blue region corresponds to weights for $F^{l}_{\downarrow 4}$, the yellow region corresponds to weights for $F^{l}_{\downarrow 8}$, and the red region corresponds to weights for $F^{l}_{\downarrow 16}$. Clear differences can be observed between weights generated from foreground and background patches.}
    \label{fig:atten_vis}
    \vspace{-1em}
\end{figure*}
\section{HyperNet Weights Visualization}

We provide additional visualizations on $\omega^{a_i,I_i}_{\mathcal{H}_\theta}$ generated from $\mathcal{H}$. There are $L=12$ layers in our search space, and each layer contains $E=10$ possible edges each with different channel numbers depend on the feature resolution. We select eight image patches from a single volume, four of which are background and the rest four are foreground. We record the corresponding $\omega^{a_i,I_i}_{\mathcal{H}_\theta}$ and plot the weight values in layer $\{1,4,12\}$ in Fig.~\ref{fig:atten_vis}. The weights are plotted following the order of the feature resolutions. We can make several observations: (1) weights in different layers have different distributions; (2) weights generated from background image patches are similar to each other within the same layer; (3) weights generated from foreground image patches are different to each other and to the background patches, within the same layer. This observation indicates that $\mathcal{H}$ learns an efficient channel-weighting mechanism that can differentiate foreground and background. We also observe that the weights for low-resolution features tend more towards 0.5, which may imply that these features are less important to learning due to their scale.
We also observe that the weights of low-resolution feature tends to be 0.5, which may imply that these features are less important for learning due to their scale. Finally, it is possible to increase the sensitivity to foreground labels by modifying $\omega^{a_i,I_i}_{\mathcal{H}_\theta}$, which may be interesting for future investigations.
